# Supplementary material for: PS4PRO: Pixel-to-pixel Supervision for Photorealistic Rendering and Optimization
Source: arXiv:2505.22616 source file (2025-05-28)
Supplement: Supplementary file 1 [file X_suppl.tex]

\clearpage
\setcounter{page}{1}
\maketitlesupplementary

\section{Implementation Details}
In this section, we provide more details on the implementation of PS4PRO and the training settings in our experiments. The first subsection introduces the detailed architecture of our model, outlining the key components and their interactions. In the following two subsections, we cover the training settings for different NeRF approaches.

\subsection{Model Architecture of PS4PRO}
The overall architecture of PS4PRO is described in Section~\ref{sec:vfi}. Our model consists of a base block and two refinement blocks. The base bock is critical in processing the input data and generating initial predictions. Then the following refinement blocks work to refine these predictions further, improving the accuracy and quality of the predictions.
% In this section, we present the details of the implementation of PS4PRO. 

\begin{figure}[h]
    \centering
    \includegraphics[width=0.35\textwidth]{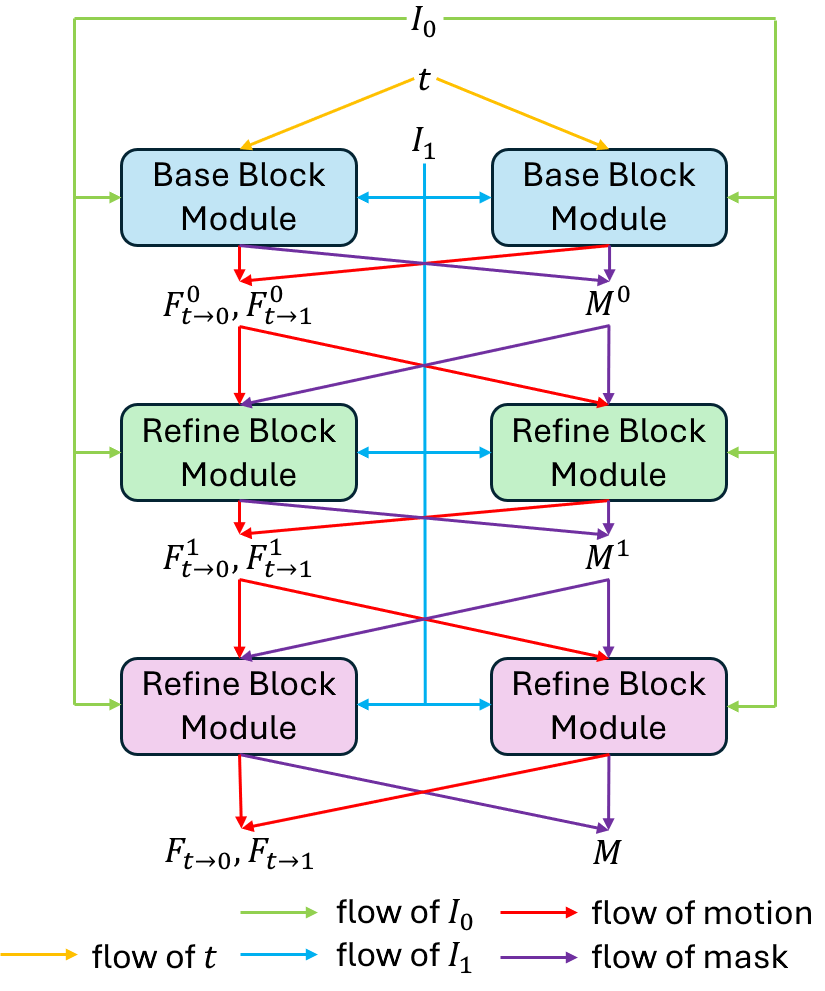}
    \caption{Detailed architecture of PS4PRO. Arrows represent the data flows between different blocks. The modules in the same color share weights.}
    \label{fig:PS4PRO}
\end{figure}

As illustrated in Figure~\ref{fig:PS4PRO}, our VFI model takes image pairs $I_0$, $I_1$, and the timestep $t$ as input. The training and inference resolution of the base block, first refinement block, and second refinement block are 1/4, 1/2, and 1 of the input resolution respectively.

In the base block, there is a pair of symmetric base block modules marked in blue, which share the same weight. The left block module takes a tensor concatenated by $I_0$, $I_1$, and $t$ as input, while the right block module takes in a tensor concatenated by $I_1$, $I_0$, and $(1-t)$. Each of the base block modules predicts a pair of motion vectors and a mask, which are then combined by taking the average to produce the output of the base block, $F^0_{t \rightarrow 0}$, $F^0_{t \rightarrow 1}$ and $M^0$.

The refinement blocks are structured similarly to the base block, consisting of a pair of symmetric refine block modules. In the first refinement block, the left block module takes a tensor concatenated by $I_0$, $I_1$, $F^0_{t \rightarrow 0}$, $F^0_{t \rightarrow 1}$, and $M^0$ as input, while the right block module takes in a tensor concatenated by $I_1$, $I_0$, $F^0_{t \rightarrow 1}$, $F^0_{t \rightarrow 0}$, and inverted $M^0$. Each of the refine block modules predicts a pair of motion vectors and a mask., which are later combined by taking the average to produce the intermediate output of the first refinement block $F^1_{t \rightarrow 0}$, $F^1_{t \rightarrow 1}$ and $M^1$.

The structure of the second refinement block is identical to that of the first one. The output motion vectors from the refine block modules in the second refinement block are combined by taking the average to produce $F_{t \rightarrow 0}$, $F_{t \rightarrow 1}$, and the average of mask outputs is the final mask $M$. These final outputs are used in Eq.~\ref{eqn:merge} to generate the novel view $I_t$ at time step $t$. 

% Notably, each module mentioned above contains two separate output groups for motion and masks, yet Figure~\ref{fig:vfi_block} showed only one in gray due to space constraints and to maintain clarity.

Notably, each block contains two submodules--one for predicting motion vectors and one for generating masks, yet Figure~\ref{fig:vfi_block} showed only one in gray due to space constraints and to maintain clarity.
We employ skip connections to enable direct information flow between these submodules and facilitate the transfer of features. This allows the submodules to share the relevant features and learn more efficiently.

% The layers of PS4PRO are reported below:

% \begin{lstlisting}[basicstyle=\tiny]
% --------------------------------------------
%   Layer (type)  Output Shape        Param #
% ============================================
%       Conv2d-1  [-1, 45, 32, 32]    3,285
%        PReLU-2  [-1, 45, 32, 32]    45
%       Conv2d-3  [-1, 90, 16, 16]    36,540
%        PReLU-4  [-1, 90, 16, 16]    90
%       Conv2d-5  [-1, 90, 16, 16]    4,500
%    LayerNorm-6  [-1, 16, 16, 90]    180
%       Linear-7  [-1, 16, 16, 180]   16,380
%         GELU-8  [-1, 16, 16, 180]   0
%       Linear-9  [-1, 16, 16, 90]    16,290
%       Block-10  [-1, 90, 16, 16]    0
%      Conv2d-11  [-1, 90, 16, 16]    4,500
%   LayerNorm-12  [-1, 16, 16, 90]    180
%      Linear-13  [-1, 16, 16, 180]   16,380
%        GELU-14  [-1, 16, 16, 180]   0
%      Linear-15  [-1, 16, 16, 90]    16,290
%       Block-16  [-1, 90, 16, 16]    0
%      Conv2d-17  [-1, 90, 16, 16]    2,340
%   LayerNorm-18  [-1, 16, 16, 90]    180
%      Linear-19  [-1, 16, 16, 180]   16,380
%        GELU-20  [-1, 16, 16, 180]   0
%      Linear-21  [-1, 16, 16, 90]    16,290
%       Block-22  [-1, 90, 16, 16]    0
%      Conv2d-23  [-1, 90, 16, 16]    2,340
%   LayerNorm-24  [-1, 16, 16, 90]    180
%      Linear-25  [-1, 16, 16, 180]   16,380
%        GELU-26  [-1, 16, 16, 180]   0
%      Linear-27  [-1, 16, 16, 90]    16,290
%       Block-28  [-1, 90, 16, 16]    0
%      Conv2d-29  [-1, 90, 16, 16]    72,990
%       PReLU-30  [-1, 90, 16, 16]    90
%      Conv2d-31  [-1, 90, 16, 16]    72,990
%       PReLU-32  [-1, 90, 16, 16]    90
%      Conv2d-33  [-1, 90, 16, 16]    72,990
%       PReLU-34  [-1, 90, 16, 16]    90
%      Conv2d-35  [-1, 90, 16, 16]    72,990
%       PReLU-36  [-1, 90, 16, 16]    90
%    ConvTr2d-37  [-1, 45, 32, 32]    64,845
%       PReLU-38  [-1, 45, 32, 32]    45
%    ConvTr2d-39  [-1, 4, 64, 64]     2,884
%    ConvTr2d-40  [-1, 45, 32, 32]    64,845
%       PReLU-41  [-1, 45, 32, 32]    45
%    ConvTr2d-42  [-1, 1, 64, 64]     721
%   BaseBlock-43 
%      Conv2d-87  [-1, 45, 64, 64]    5,310
%       PReLU-88  [-1, 45, 64, 64]    45
%      Conv2d-89  [-1, 90, 32, 32]    36,540
%       PReLU-90  [-1, 90, 32, 32]    90
%      Conv2d-91  [-1, 90, 32, 32]    72,990
%       PReLU-92  [-1, 90, 32, 32]    90
%      Conv2d-93  [-1, 90, 32, 32]    72,990
%       PReLU-94  [-1, 90, 32, 32]    90
%      Conv2d-95  [-1, 90, 32, 32]    72,990
%       PReLU-96  [-1, 90, 32, 32]    90
%      Conv2d-97  [-1, 90, 32, 32]    72,990
%       PReLU-98  [-1, 90, 32, 32]    90
%      Conv2d-99  [-1, 90, 32, 32]    72,990
%      PReLU-100  [-1, 90, 32, 32]    90
%     Conv2d-101  [-1, 90, 32, 32]    72,990
%      PReLU-102  [-1, 90, 32, 32]    90
%     Conv2d-103  [-1, 90, 32, 32]    72,990
%      PReLU-104  [-1, 90, 32, 32]    90
%     Conv2d-105  [-1, 90, 32, 32]    72,990
%      PReLU-106  [-1, 90, 32, 32]    90
%   ConvTr2d-107  [-1, 45, 64, 64]    64,845
%      PReLU-108  [-1, 45, 64, 64]    45
%   ConvTr2d-109  [-1, 4, 128, 128]   2,884
%   ConvTr2d-110  [-1, 45, 64, 64]    64,845
%      PReLU-111  [-1, 45, 64, 64]    45
%   ConvTr2d-112  [-1, 1, 128, 128]   721
%   RefBlock-113  
%     Conv2d-141  [-1, 45, 128, 128]  5,310
%      PReLU-142  [-1, 45, 128, 128]  45
%     Conv2d-143  [-1, 90, 64, 64]    36,540
%      PReLU-144  [-1, 90, 64, 64]    90
%     Conv2d-145  [-1, 90, 64, 64]    72,990
%      PReLU-146  [-1, 90, 64, 64]    90
%     Conv2d-147  [-1, 90, 64, 64]    72,990
%      PReLU-148  [-1, 90, 64, 64]    90
%     Conv2d-149  [-1, 90, 64, 64]    72,990
%      PReLU-150  [-1, 90, 64, 64]    90
%     Conv2d-151  [-1, 90, 64, 64]    72,990
%      PReLU-152  [-1, 90, 64, 64]    90
%     Conv2d-153  [-1, 90, 64, 64]    72,990
%      PReLU-154  [-1, 90, 64, 64]    90
%     Conv2d-155  [-1, 90, 64, 64]    72,990
%      PReLU-156  [-1, 90, 64, 64]    90
%     Conv2d-157  [-1, 90, 64, 64]    72,990
%      PReLU-158  [-1, 90, 64, 64]    90
%     Conv2d-159  [-1, 90, 64, 64]    72,990
%      PReLU-160  [-1, 90, 64, 64]    90
%   ConvTr2d-161  [-1, 45, 128, 128]  64,845
%      PReLU-162  [-1, 45, 128, 128]  45
%   ConvTr2d-163  [-1, 4, 256, 256]   2,884
%   ConvTr2d-164  [-1, 45, 128, 128]  64,845
%      PReLU-165  [-1, 45, 128, 128]  45
%   ConvTr2d-166  [-1, 1, 256, 256]   721
%   RefBlock-167  
% --------------------------------------------
% \end{lstlisting}

\subsection{Training Settings for Lightning-NeRF}
\label{sec:lnerf_sup}
In this subsection, we provide the training settings used for the Lightning-NeRF approach \cite{cao2024lightning}.
For the experiment in Section~\ref{sec::neurand}, we trained Lightning-NeRF on Argoverse2 \cite{argoverse} dataset using the setting below:

\begin{lstlisting}[basicstyle=\tiny]
    --max-num-iterations 30001 
    --machine.num-gpus 1 
    --vis tensorboard 
    --mixed-precision True 
    --experiment-name baseline 
    --timestamp 098fe60e-bab0-32e2-89bc-bedced881911 
    --steps-per-eval-all-images 5000 
    --pipeline.model.frontal-axis x 
    --pipeline.datamanager.train-num-rays-per-batch 32768 
    --pipeline.model.init-density-value 10.0 
    --pipeline.model.density-grid-base-res 256 
    --pipeline.model.density-log2-hashmap-size 24 
    --pipeline.model.bg-density-grid-res 32 
    --pipeline.model.bg-density-log2-hashmap-size 18 
    --pipeline.model.near-plane 0.01 
    --pipeline.model.far-plane 10.0 
    --pipeline.model.vi-mlp-num-layers 3 
    --pipeline.model.vi-mlp-hidden-size 64 
    --pipeline.model.vd-mlp-num-layers 2 
    --pipeline.model.vd-mlp-hidden-size 32 
    --pipeline.model.color-grid-base-res 128 
    --pipeline.model.color-grid-max-res 2048 
    --pipeline.model.color-grid-fpl 2 
    --pipeline.model.color-grid-num-levels 8 
    --pipeline.model.bg-color-grid-base-res 32 
    --pipeline.model.bg-color-grid-max-res 128 
    --pipeline.model.bg-color-log2-hashmap-size 16 
    --pipeline.model.alpha-thre 0.02 
    --pipeline.model.occ-grid-base-res 256 
    --pipeline.model.occ-grid-num-levels 4 
    --pipeline.model.occ-num-samples-per-ray 750 
    --pipeline.model.occ-grid-update-warmup-step 2 
    --pipeline.model.pdf-num-samples-per-ray 8 
    --pipeline.model.pdf-samples-warmup-step 1000 
    --pipeline.model.pdf-samples-fixed-step 3000 
    --pipeline.model.pdf-samples-fixed-ratio 0.5 
    --pipeline.model.appearance-embedding-dim 0 
    --pipeline.datamanager.train-num-images-to-sample-from 128 
    --pipeline.datamanager.train-num-times-to-repeat-images 256 
\end{lstlisting}

Since the VFI methods are only trained on the Vimeo90K dataset, which has an aspect ratio of 4:3, we applied a 4:3 mask on the interpolated result where they are used to reconstruct the 3D scene. In Section~\ref{sec::neurand} we trained Lightning-NeRF on KITTI \cite{liao2022kitti} dataset using the setting below:

\begin{lstlisting}[basicstyle=\tiny]
    --max-num-iterations 30001
    --machine.num-gpus 1
    --vis tensorboard 
    --mixed-precision True 
    --steps-per-eval-all-images 5000 
    --pipeline.model.frontal-axis x 
    --pipeline.datamanager.train-num-rays-per-batch 65536 
    --pipeline.model.init-density-value 10.0 
    --pipeline.model.density-grid-base-res 256 
    --pipeline.model.density-log2-hashmap-size 24 
    --pipeline.model.bg-density-grid-res 32 
    --pipeline.model.bg-density-log2-hashmap-size 18 
    --pipeline.model.near-plane 0.01 
    --pipeline.model.far-plane 6.0 
    --pipeline.model.vi-mlp-num-layers 3 
    --pipeline.model.vi-mlp-hidden-size 64
    --pipeline.model.vd-mlp-num-layers 2 
    --pipeline.model.vd-mlp-hidden-size 32
    --pipeline.model.color-grid-base-res 128 
    --pipeline.model.color-grid-max-res 2048 
    --pipeline.model.color-grid-fpl 2 
    --pipeline.model.color-grid-num-levels 8 
    --pipeline.model.bg-color-grid-base-res 32
    --pipeline.model.bg-color-grid-max-res 128 
    --pipeline.model.bg-color-log2-hashmap-size 16 
    --pipeline.model.alpha-thre 0.01 
    --pipeline.model.occ-grid-base-res 256 
    --pipeline.model.occ-grid-num-levels 2 
    --pipeline.model.occ-num-samples-per-ray 750 
    --pipeline.model.occ-grid-update-warmup-step 256 
    --pipeline.model.pdf-num-samples-per-ray 8 
    --pipeline.model.pdf-samples-warmup-step 100000 
    --pipeline.model.pdf-samples-fixed-step 100000 
    --pipeline.model.pdf-samples-fixed-ratio 0.5 
    --pipeline.model.appearance-embedding-dim 0 
    --pipeline.datamanager.train-num-images-to-sample-from 128 
    --pipeline.datamanager.train-num-times-to-repeat-images 256 
\end{lstlisting}

\subsection{Training Settings for Neurad}
In Section~\ref{sec::neurand}, we trained NeuRAD \cite{neurad} on NuScenes-mini \cite{nuscenes} dataset using the setting below:

\begin{lstlisting}[basicstyle=\tiny]
    --max-num-iterations 60001 
    --machine.num-devices 1
    --pipeline.model.eval_num_rays_per_chunk 65536 
    --pipeline.datamanager.num_processes 8 
    --pipeline.datamanager.train-num-lidar-rays-per-batch 32768 
    --pipeline.datamanager.eval-num-lidar-rays-per-batch 16384 
    --pipeline.datamanager.train-num-rays-per-batch 65536 
    --pipeline.datamanager.eval-num-rays-per-batch 65536 
    --pipeline.datamanager.train-num-images-to-sample-from 128 
    --pipeline.datamanager.train-num-times-to-repeat-images 256 
    --optimizers.trajectory-opt.scheduler.warmup-steps 1 
    --optimizers.trajectory-opt.scheduler.max-steps 2 
    --pipeline.model.field.grid.actor.flip-prob 0.5 
    --pipeline.model.sampling.proposal-field-1.grid.actor.flip-prob 0.5 
    --pipeline.model.sampling.proposal-field-2.grid.actor.flip-prob 0.5 
    --pipeline.model.camera-optimizer.mode SO3xR3
    --vis tensorboard
\end{lstlisting}

\section{Supplementary Experiment}
\subsection{Speed and Model Size Comparison}

To evaluate the speed and efficiency of PS4PRO and other methods, we compared the runtime of all VFI methods on three different input resolutions $1024 \times 512$ (0.5MP), $2048 \times 1024$ (2.1MP), and $4096 \times 2048$ (8.4MP) on an NVIDIA RTX 3090. 

Table~\ref{tab:speed} presents the runtime of tested methods in milliseconds. EMA-s has a notably longer runtime than the others, while RIFE demonstrates the fastest runtime. Our model achieves the second fastest runtime with the smallest parameter size, indicating that our method is compact in architecture and efficient in computation.

\begin{table}[h]
  \vspace{-0.3cm}
  \
  \vspace{-0.2cm}
  \begin{tabular}{l c c c c}
    \toprule
    Method & Parameters & 0.5MP & 2.1MP & 8.4MP \\
    \midrule
    M2M & 7.61M & 21.32ms & 63.29ms & 230.9ms\\
    IFRNet & \underline{4.96M}  & 14.01ms & 52.12ms & 234.3ms\\
    RIFE & 10.7M & \textbf{12.04ms} & \textbf{44.05ms} & \textbf{182.3ms}\\
    EMA-s & 14.3M & 27.91ms & 119.5ms & 410.8ms\\
    Ours & \textbf{5.09M} & \underline{13.03ms} & \underline{50.32ms} & \underline{208.9ms}\\
    \bottomrule
  \end{tabular}
  \caption{Comparison of model size (in millions, M) and runtime (in milliseconds, ms) of different methods on various input resolutions.}
  \vspace{-0.4cm}
  \label{tab:speed}
\end{table}

\subsection{Comparison with diffusion method}

The diffusion-based methods have recently demonstrated their ability to generate high-quality novel views from ultra-sparse input images. In Table~\ref{tab:viewcrafter}, we compare the performance of our model with that of a diffusion-based approach in terms of efficiency. We perform data augmentation using ViewCrafter \cite{yu2024viewcrafter} to generate one novel view between each training image in the KITTI dataset. The time for performing augmentation to generate one new frame between each training image and the proportion of augmentation time over the entire neural rendering process is reported in Table~\ref{tab:viewcrafter}. As demonstrated, our data augmentation method PS4PRO has negligible runtime compared to the 3D reconstruction time, whereas the diffusion time using ViewCrafter is $5.88\times$ the 3D reconstruction time. Therefore, our method is more practical and better suited for integration into the neural rendering pipeline as a part of the pixel sampler, providing both high-quality predictions and improved computational efficiency.

\begin{table}[h]
  \centering
  \begin{tabular}{l c c c}
    \toprule
    Method & Parameters & Aug. Time & Ratio to Training\\
    \midrule
    ViewCrafter & 3106M & 79,848s & 588\%\\
    PS4PRO & 5.09M & 7.69s & 0.057\% \\
    \bottomrule
  \end{tabular}
  \caption{Comparison of PS4PRO against ViewCrafter in terms of computation cost and efficiency on KITTI dataset.}
  \label{tab:viewcrafter}
\end{table}

\begin{figure*}[h!]
    \centering
    \includegraphics[width=0.98\textwidth]{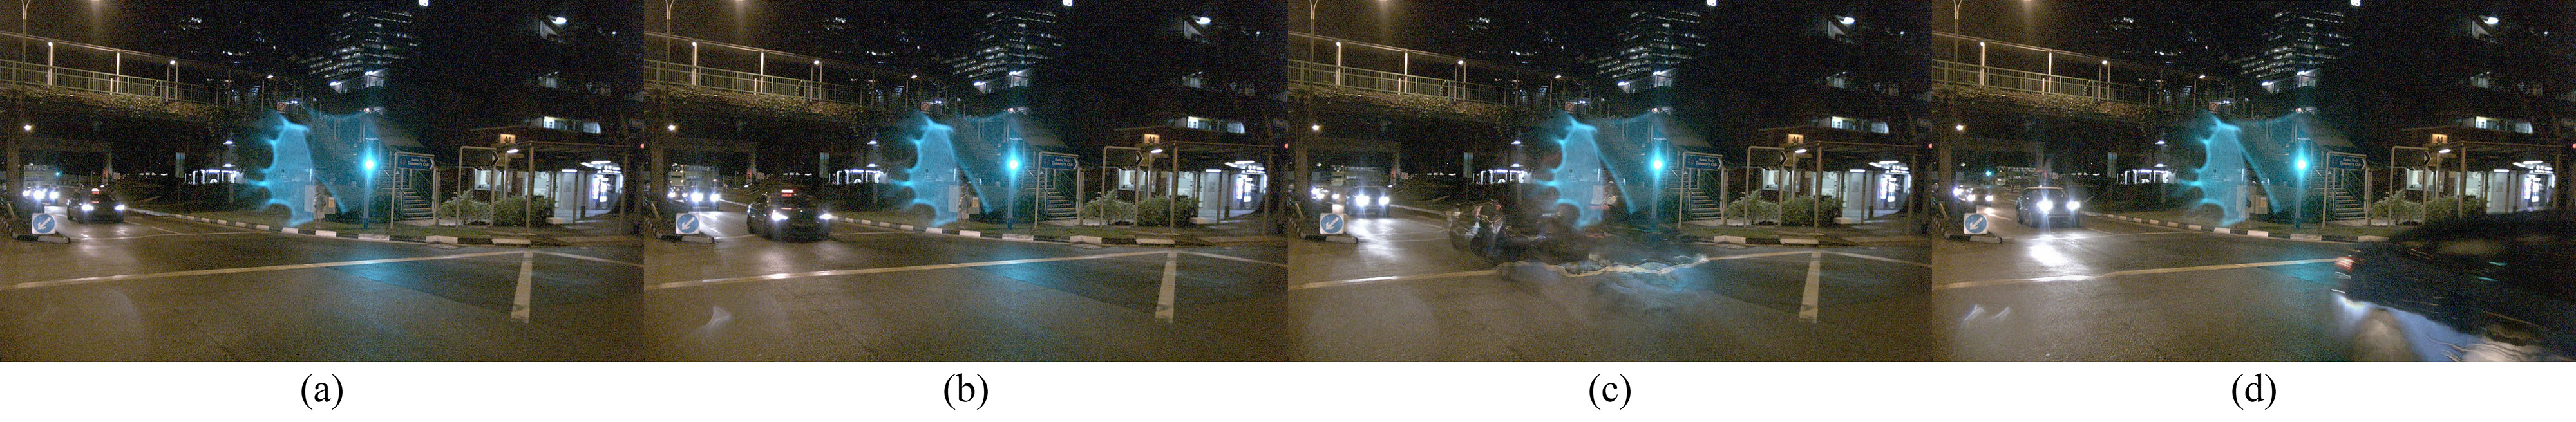}
    \caption{A failure case produced by PS4PRO, where all four images are generated as interpolation results. (a), (b), (c), and (d) correspond to timestamps 1542801004012460, 1542801004812460, 1542801005612460, and 1542801006512460 in the NuScenes dataset respectively.}
    \label{fig:fail}
\end{figure*}

\section{Failure Case}
Through the experiments we have performed in Section~\ref{sec::neurand}, we have noticed that our proposed method can be further improved where a strong disturbance exists. As shown in Figure~\ref{fig:fail}, PS4PRO fails at the certain timestamp (c) when the car passes the area possessed by the glare of the traffic light. Dominated by the priority to match the closest patterns, PS4PRO superposes the glare in the position of the car, interfering with the accurate representation.
